# Supplementary material for: Fully numerical electronic structure calculations on diatomic molecules in weak to strong magnetic fields
Source: arXiv:1812.06274 source file (2019-02-19)
Supplement: Supplementary file 1 [file SI.pdf]

# Supporting Information: Fully numerical electronic structure calculations on diatomic molecules in weak and strong magnetic fields

Susi Lehtola, Maria Dimitrova, and Dage Sundholm

Department of Chemistry, University of Helsinki, P.O. Box 55 (A. I. Virtasen aukio 1),  
FI-00014 University of Helsinki, Finland

## ARTICLE HISTORY

Compiled February 17, 2019

The total energy as a function of the magnetic field strength for all states obtained in the calculations with the finite-element (FEM) calculations with HELFEM, and the gauge-including Gaussian-type orbital (GTO) calculations with LONDON are shown in Figs. 1 to 2 for  $\text{H}_2$ , in Figs. 3 to 4 for  $\text{HeH}^+$ , in Figs. 5 to 7 for  $\text{LiH}$ , in Figs. 8 to 10 for  $\text{BeH}^+$ , in Figs. 11 to 13 for  $\text{BH}$ , and in Figs. 14 to 16 for  $\text{CH}^+$ . The resulting ground-state configurations in the FEM and GTO calculations have been identified in table 1 for  $\text{H}_2$ ,  $\text{HeH}^+$ , and  $\text{LiH}$ , and in tables 2, 3 and 4 for  $\text{BeH}^+$ ,  $\text{BH}$  and  $\text{CH}^+$ , respectively.

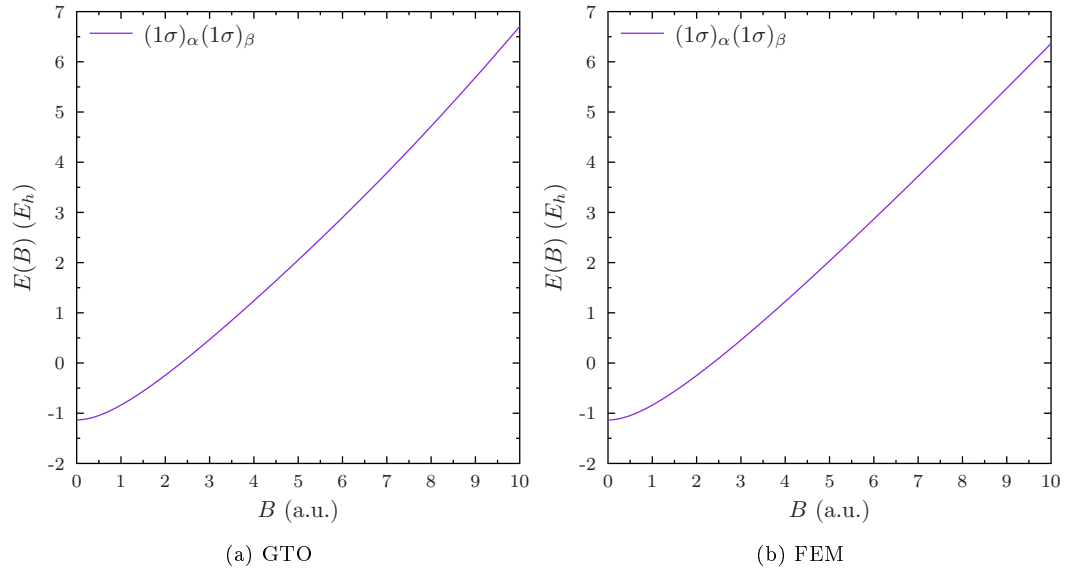

Figure 1.:  $H_2$  singlet.

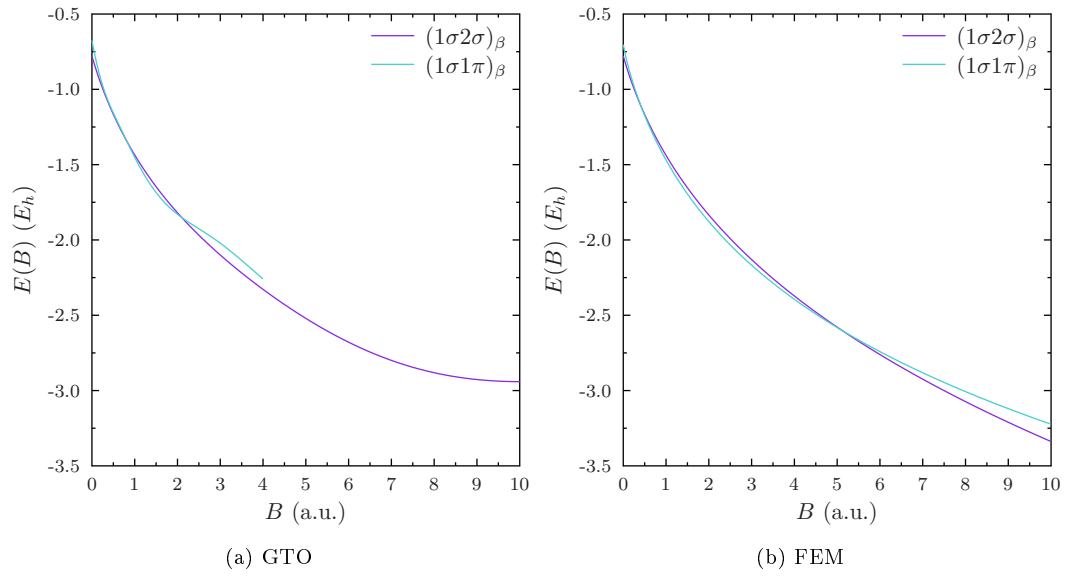

Figure 2.:  $H_2$  triplet.

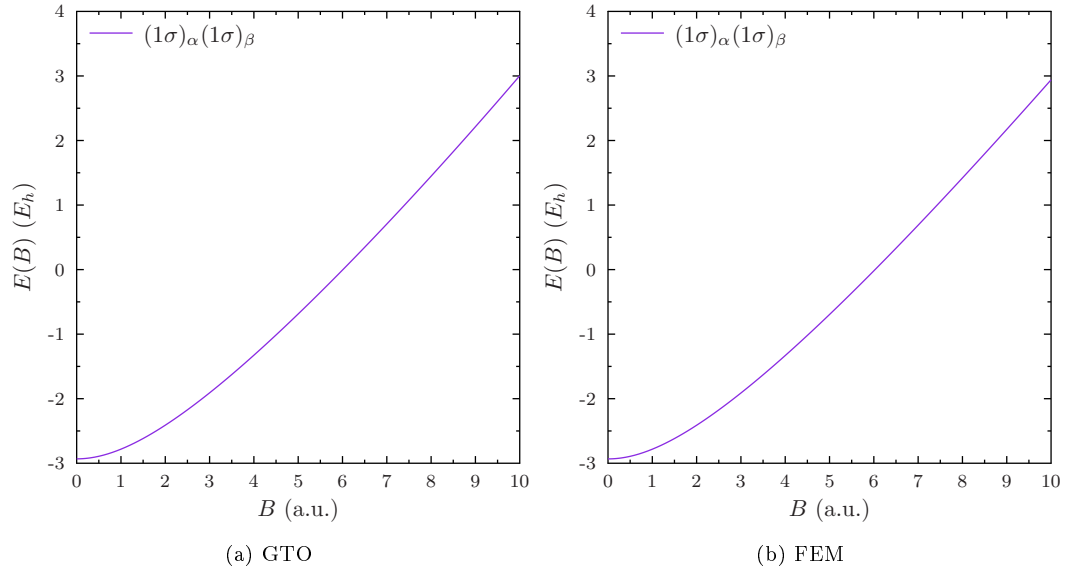

Figure 3.:  $\text{HeH}^+$  singlet.

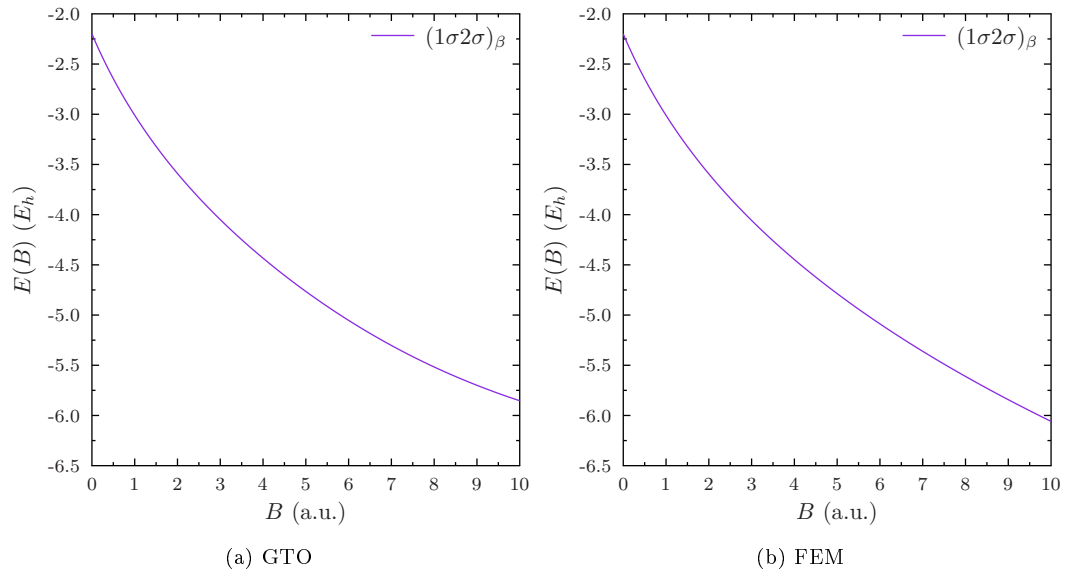

Figure 4.:  $\text{HeH}^+$  triplet.

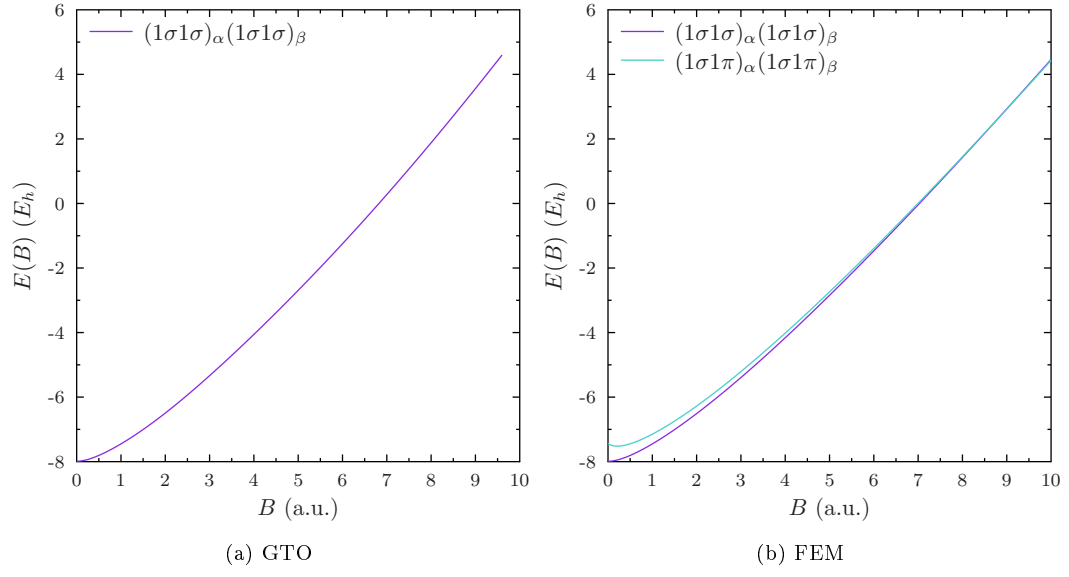

Figure 5.: LiH singlet.

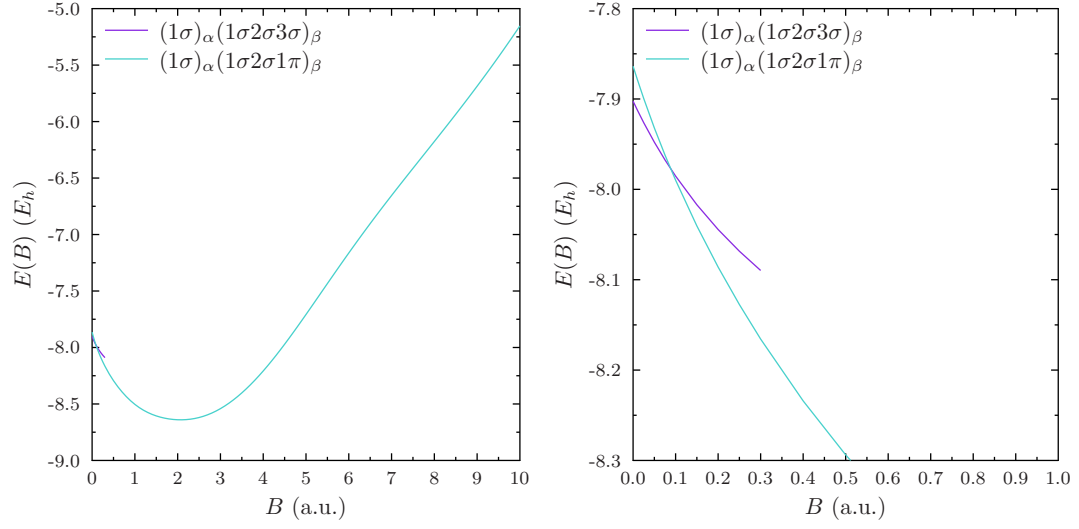

(a) GTO

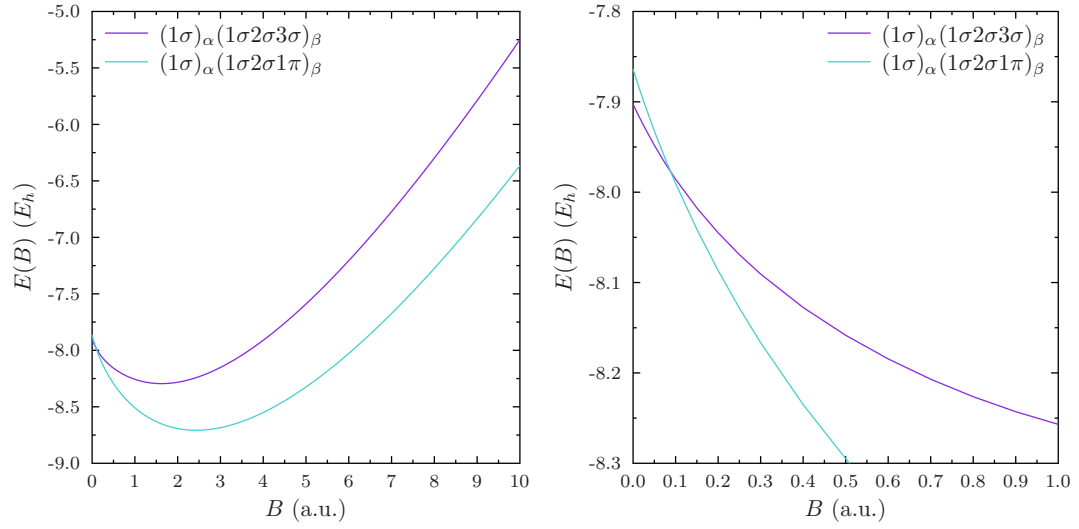

(b) FEM

Figure 6.: LiH triplet.

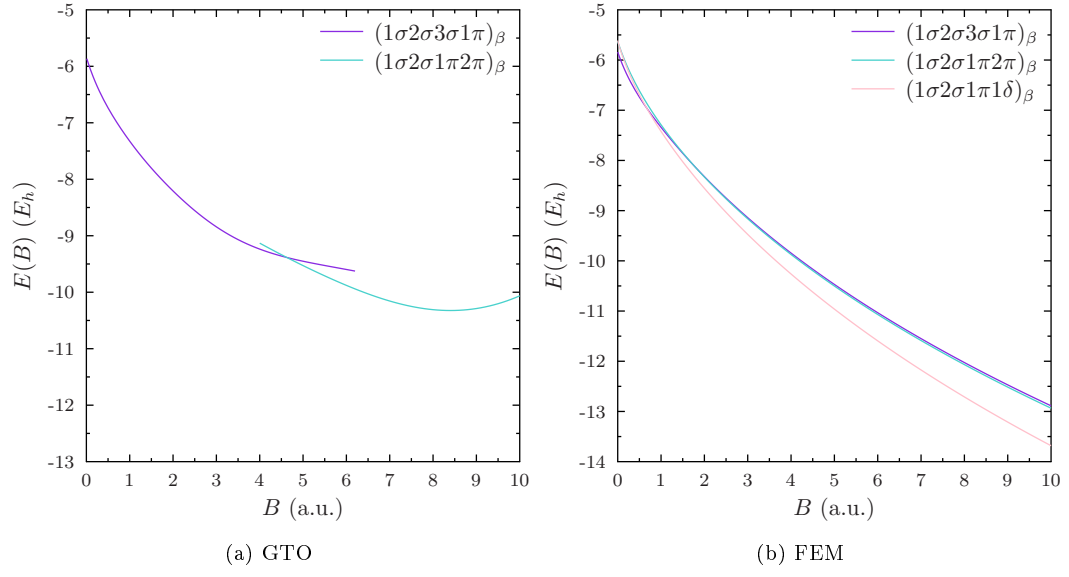

Figure 7.: LiH quintet.

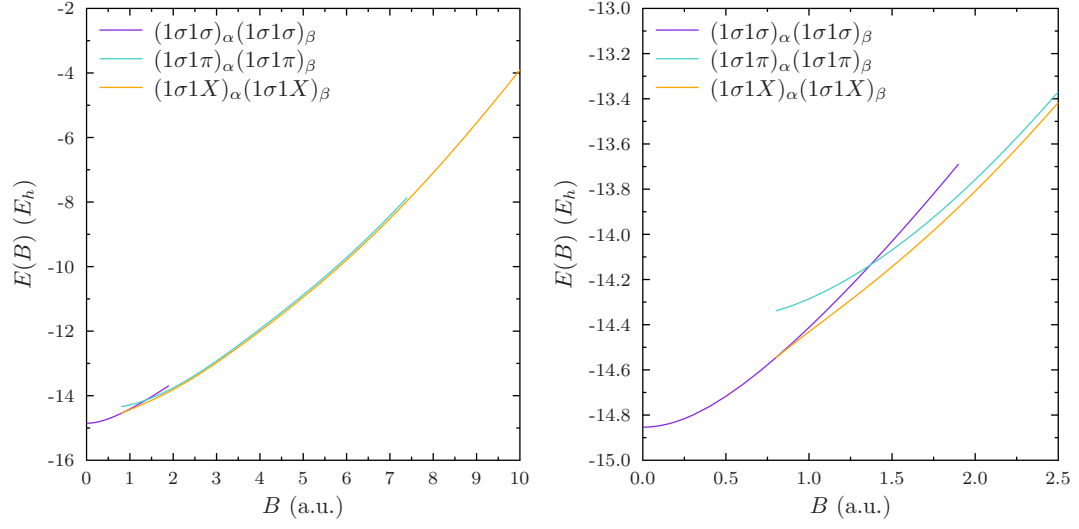

(a) GTO

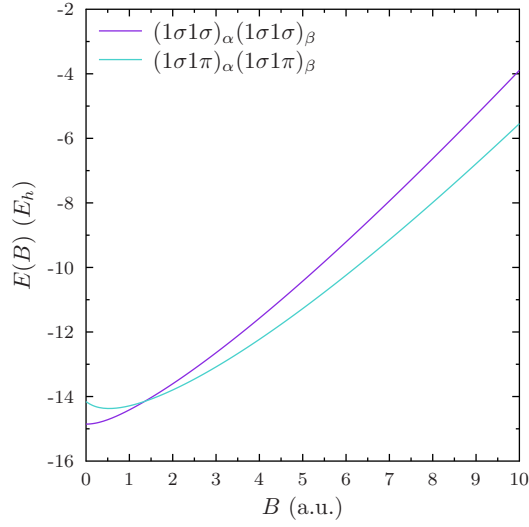

(b) FEM

Figure 8.:  $\text{BeH}^+$  singlet.

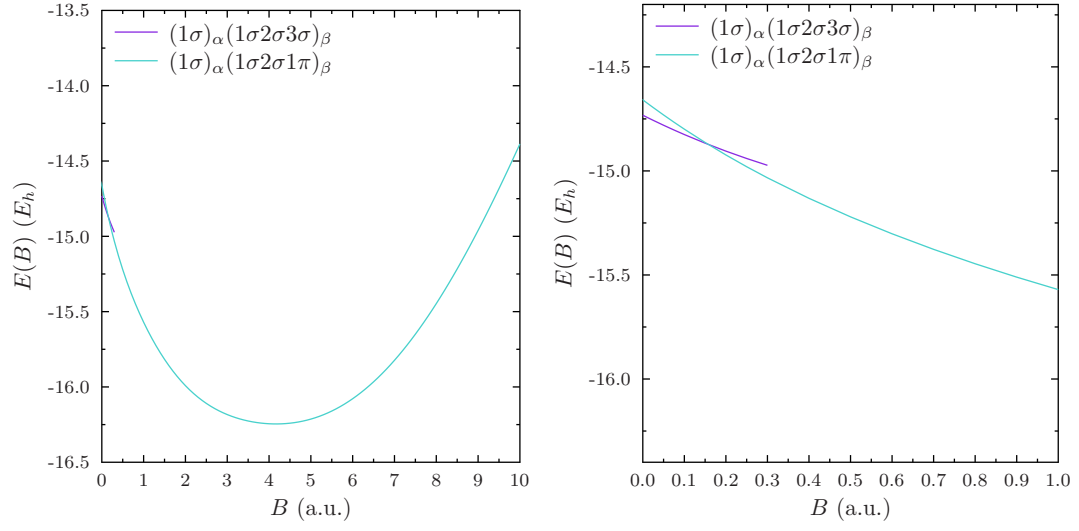

(a) GTO

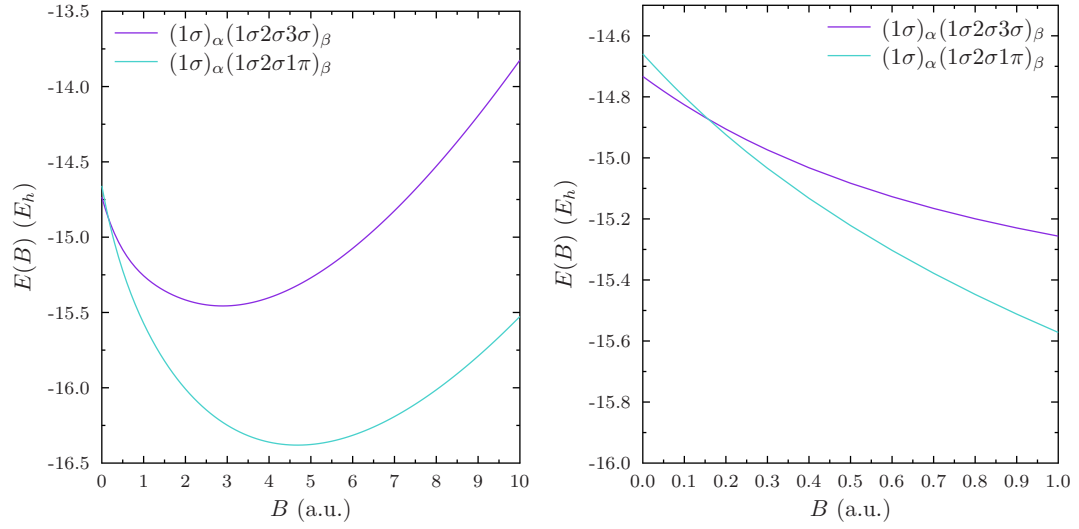

(b) FEM

Figure 9.:  $\text{BeH}^+$  triplet.



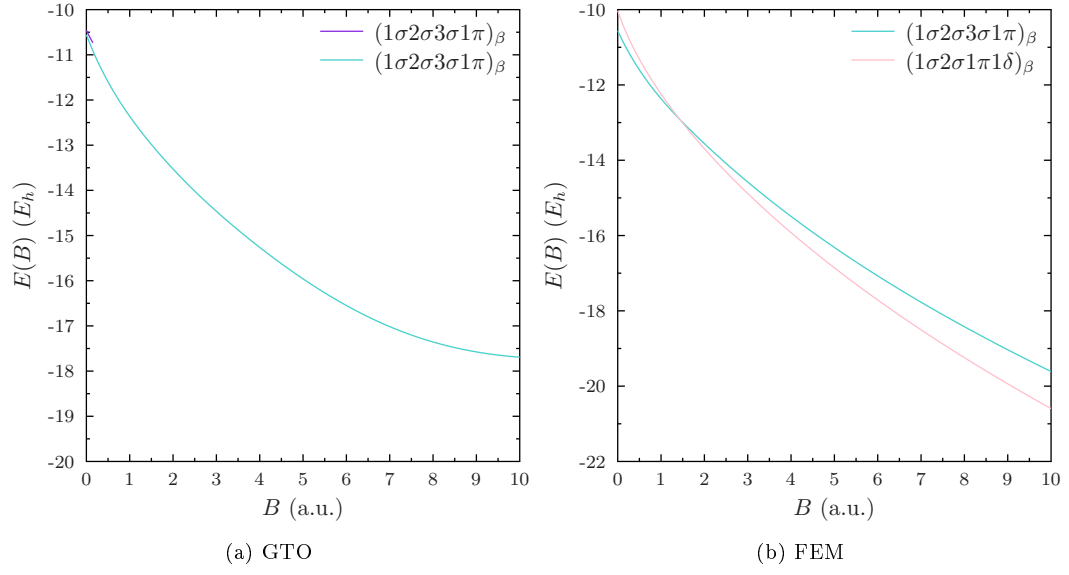

Figure 10.:  $\text{BeH}^+$  quintet.

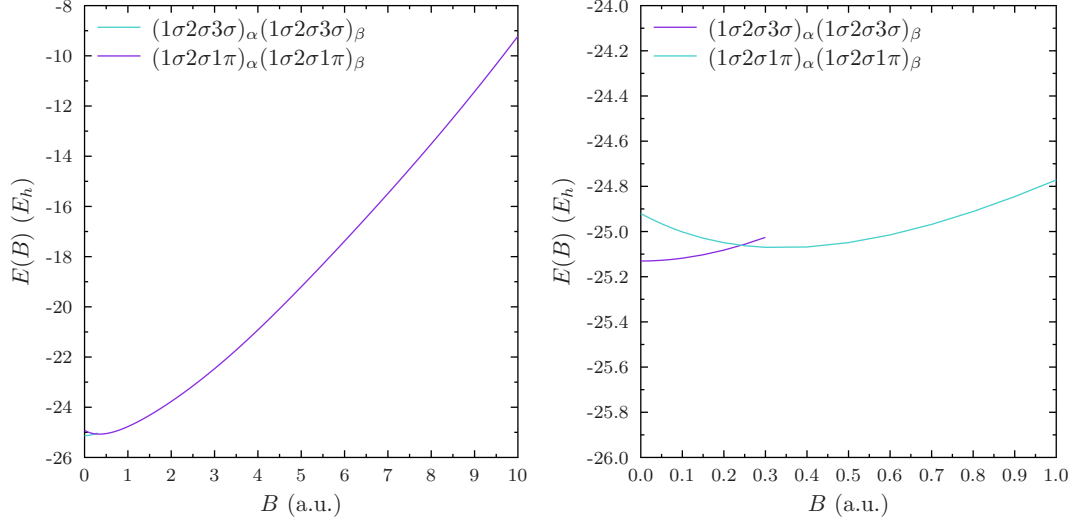

(a) GTO

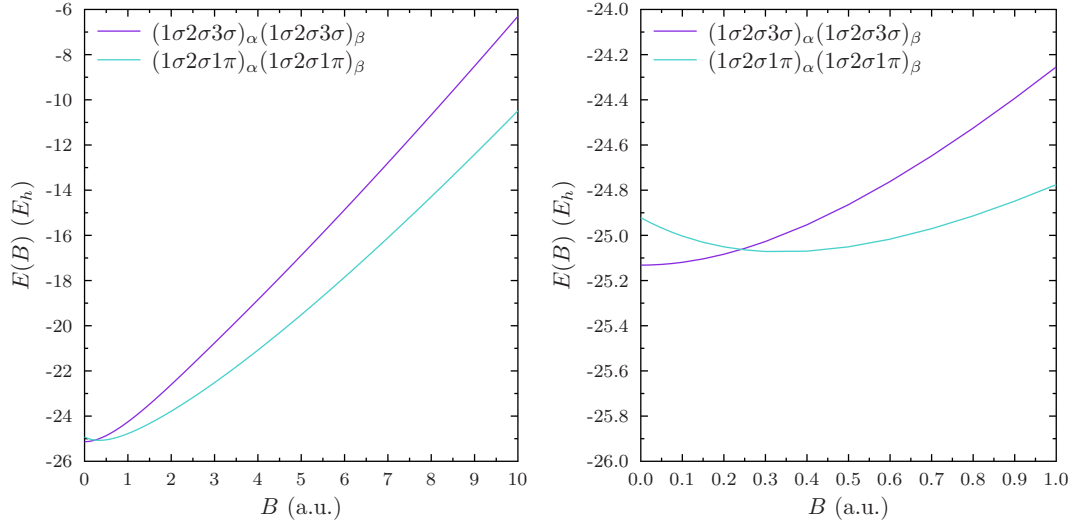

(b) FEM

Figure 11.: BH singlet.

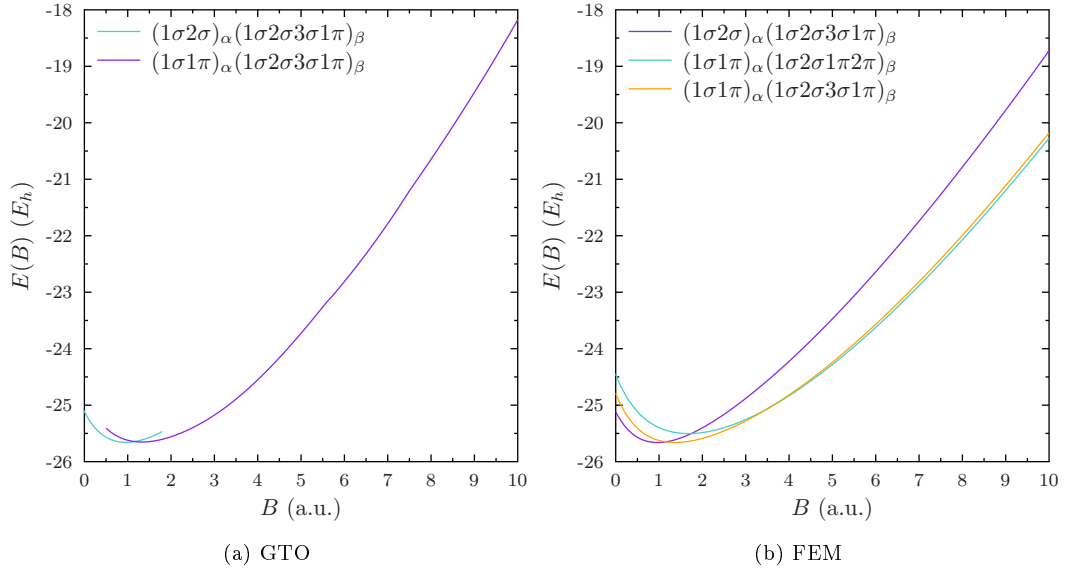

Figure 12.: BH triplet.

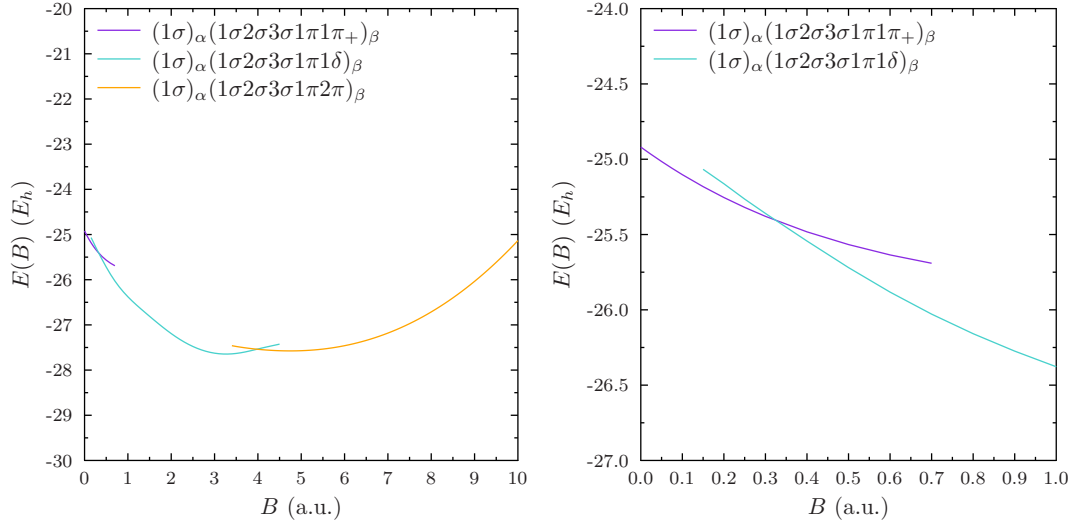

(a) GTO

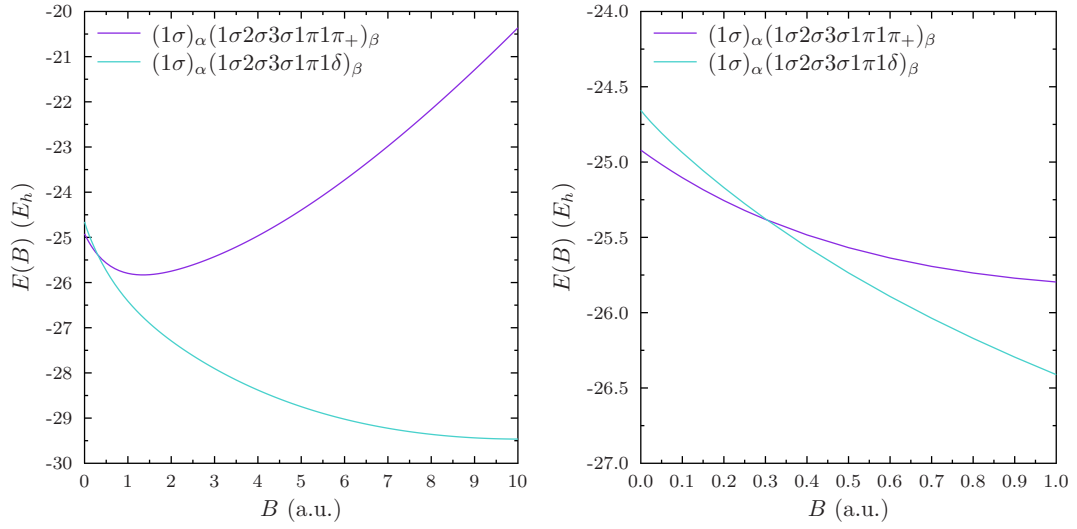

(b) FEM

Figure 13.: BH quintet.

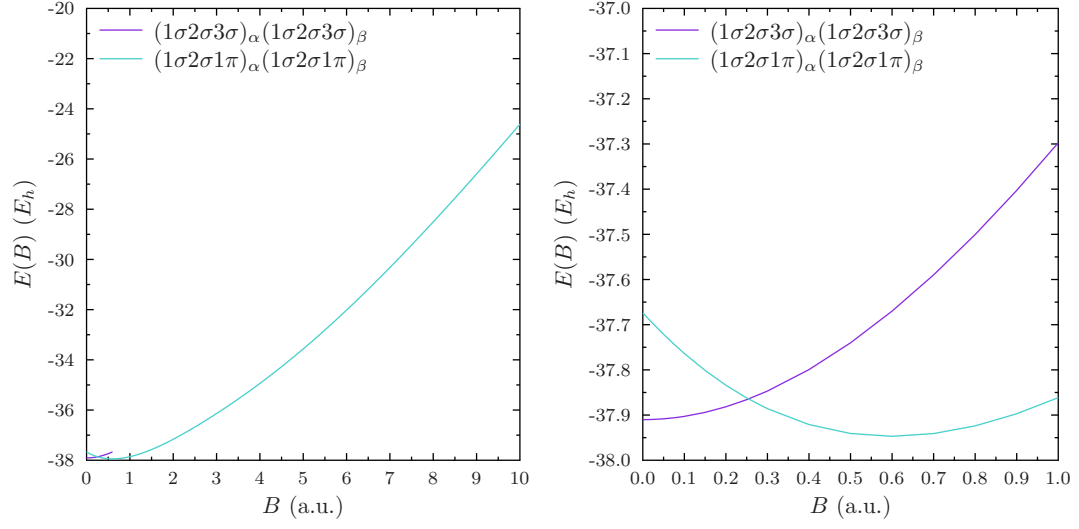

(a) GTO

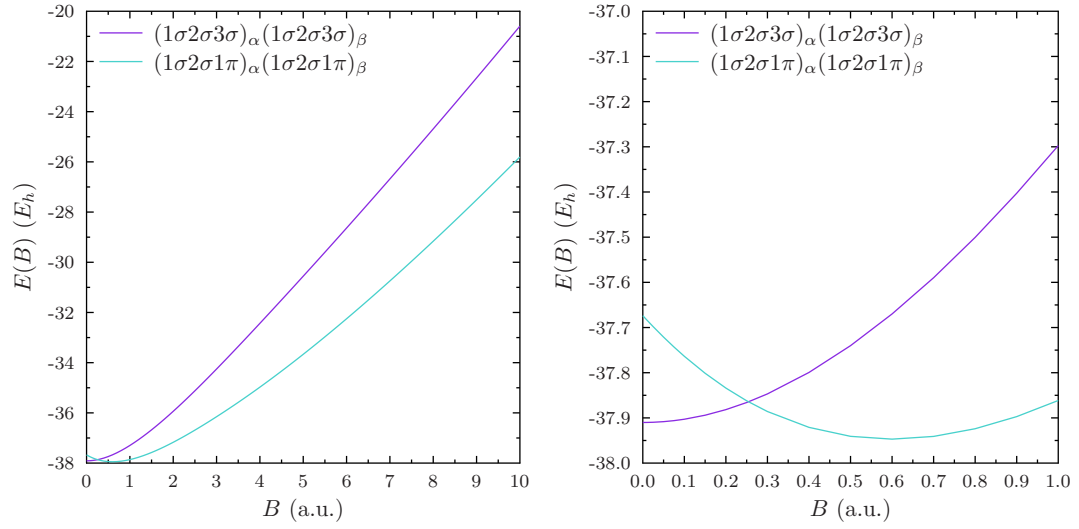

(b) FEM

Figure 14.:  $\text{CH}^+$  singlet.

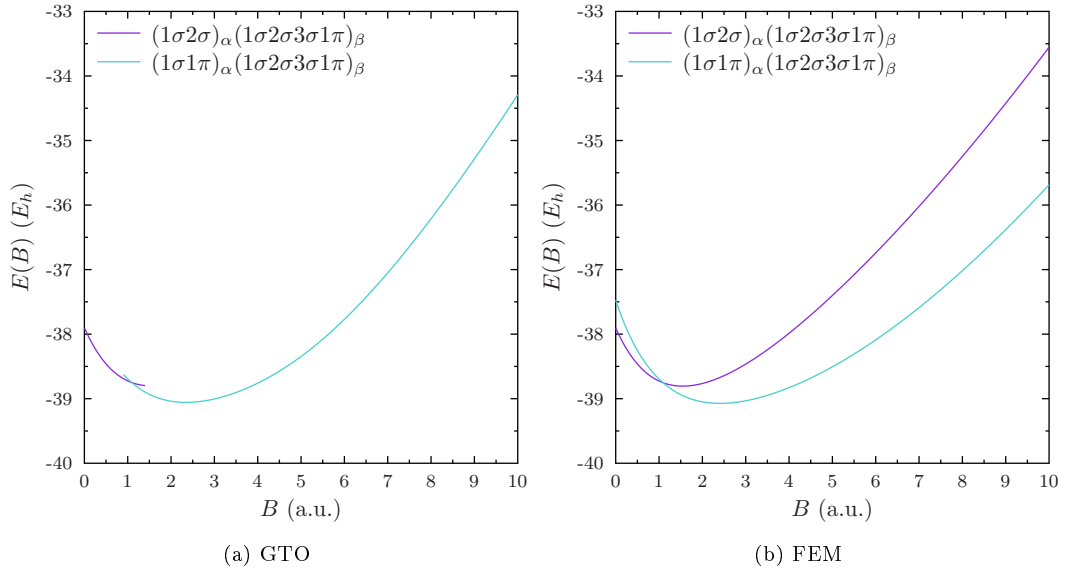

Figure 15.:  $\text{CH}^+$  triplet.

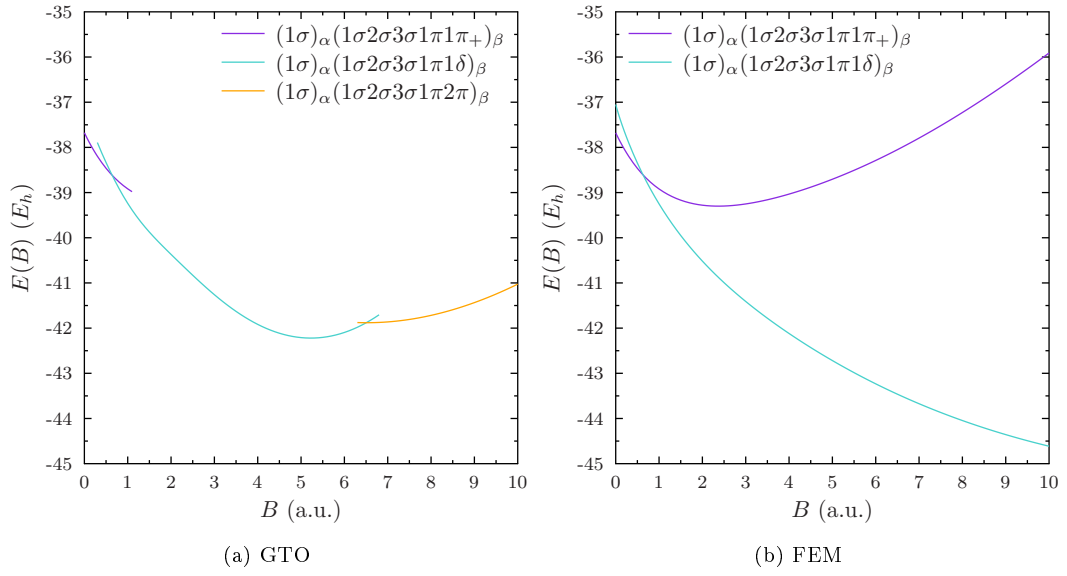

Figure 16.:  $\text{CH}^+$  quintet.

Table 1.: Ground-state configurations for  $\text{H}_2$ ,  $\text{HeH}^+$ ,  $\text{LiH}$ , and  $\text{BeH}^+$  as a function of the magnetic field strength calculated at the Hartree–Fock level using gauge-including Gaussian-type orbitals (GTO) and finite element (FEM) basis sets. The label X refers to symmetry-broken orbitals. Note that the orbitals are not sorted according to their energies.

| Molecule       | spin state | basis | configuration                                      | field strength ( $B_0$ ) |
|----------------|------------|-------|----------------------------------------------------|--------------------------|
| $\text{H}_2$   | singlet    | FEM   | $1\sigma_\alpha 1\sigma_\beta$                     | $0 \leq B \leq 10$       |
|                |            | GTO   | $1\sigma_\alpha 1\sigma_\beta$                     | $0 \leq B \leq 10$       |
|                | triplet    | FEM   | $(1\sigma 2\sigma)_\beta$                          | $0 \leq B < 0.5$         |
|                |            |       | $(1\sigma 1\pi)_\beta$                             | $0.5 \leq B < 5.2$       |
|                |            |       | $(1\sigma 2\sigma)_\beta$                          | $5.2 \leq B \leq 10$     |
|                |            | GTO   | $(1\sigma 2\sigma)_\beta$                          | $0 \leq B < 0.9$         |
|                |            |       | $(1\sigma 1\pi)_\beta$                             | $0.9 \leq B < 2.2$       |
|                |            |       | $(1\sigma 2\sigma)_\beta$                          | $2.2 \leq B \leq 10$     |
| $\text{HeH}^+$ | singlet    | FEM   | $1\sigma_\alpha 1\sigma_\beta$                     | $0 \leq B \leq 10$       |
|                |            | GTO   | $1\sigma_\alpha 1\sigma_\beta$                     | $0 \leq B \leq 10$       |
|                | triplet    | FEM   | $(1\sigma 2\sigma)_\beta$                          | $0 \leq B \leq 10$       |
|                |            | GTO   | $(1\sigma 2\sigma)_\beta$                          | $0 \leq B \leq 10$       |
| $\text{LiH}$   | singlet    | FEM   | $(1\sigma 2\sigma)_\alpha (1\sigma 2\sigma)_\beta$ | $0 \leq B < 8.8$         |
|                |            |       | $(1\sigma 1\pi)_\alpha (1\sigma 1\pi)_\beta$       | $8.8 \leq B \leq 10$     |
|                |            | GTO   | $(1\sigma 2\sigma)_\alpha (1\sigma 2\sigma)_\beta$ | $0 \leq B < 9.6$         |
|                |            |       | $(1\sigma X)_\alpha (1\sigma X)_\beta$             | $9.6 \leq B \leq 10$     |
|                | triplet    | FEM   | $1\sigma_\alpha (1\sigma 2\sigma 3\sigma)_\beta$   | $0 \leq B < 0.1$         |
|                |            |       | $1\sigma_\alpha (1\sigma 2\sigma 3\sigma)_\beta$   | $0.1 \leq B \leq 10$     |
|                |            | GTO   | $1\sigma_\alpha (1\sigma 2\sigma 3\sigma)_\beta$   | $0 \leq B < 0.1$         |
|                |            |       | $1\sigma_\alpha (1\sigma 2\sigma 1\pi)_\beta$      | $0.1 \leq B \leq 10$     |
|                | quintet    | FEM   | $(1\sigma 2\sigma 3\sigma 1\pi)_\beta$             | $0 \leq B < 0.1$         |
|                |            |       | $(1\sigma 2\sigma 1\pi 3\sigma)_\beta$             | $0.1 \leq B < 0.7$       |
|                |            |       | $(1\sigma 2\sigma 1\pi 1\delta)_\beta$             | $0.7 \leq B < 2.0$       |
|                |            |       | $(1\sigma 1\pi 2\sigma 1\delta)_\beta$             | $2.0 \leq B \leq 10$     |
|                |            | GTO   | $(1\sigma 2\sigma 3\sigma 4\sigma)_\beta$          | $0 \leq B < 0.01$        |
|                |            |       | $(1\sigma 2\sigma 3\sigma 1\pi)_\beta$             | $0.01 \leq B < 4.7$      |
|                |            |       | $(1\sigma 2\sigma 1\pi 2\pi)_\beta$                | $4.7 \leq B < 9.7$       |
|                |            |       | $(1\sigma 2\sigma 3\sigma 1\pi)_\beta$             | $9.7 \leq B \leq 10$     |

Table 2.: Ground-state configurations for  $\text{BeH}^+$  as a function of the magnetic field strength calculated at the Hartree–Fock level using gauge-including Gaussian-type orbitals (GTO) and finite element (FEM) basis sets.

| Spin state | basis | configuration                                      | field strength ( $B_0$ ) |
|------------|-------|----------------------------------------------------|--------------------------|
| singlet    | FEM   | $(1\sigma 2\sigma)_\alpha (1\sigma 2\sigma)_\beta$ | $0 \leq B < 1.4$         |
|            |       | $(1\sigma 1\pi)_\alpha (1\sigma 1\pi)_\beta$       | $1.4 \leq B < 10$        |
|            | GTO   | $(1\sigma 2\sigma)_\alpha (1\sigma 2\sigma)_\beta$ | $0 \leq B < 1.4$         |
|            |       | $(1\sigma 1\pi)_\alpha (1\sigma 1\pi)_\beta$       | $1.4 \leq B \leq 10$     |
| triplet    | FEM   | $1\sigma_\alpha (1\sigma 2\sigma 3\sigma)_\beta$   | $0 \leq B < 0.2$         |
|            |       | $1\sigma_\alpha (1\sigma 2\sigma 1\pi)_\beta$      | $0.2 \leq B < 2.0$       |
|            |       | $1\sigma_\alpha (1\sigma 1\pi 2\sigma)_\beta$      | $2.0 \leq B < 10$        |
|            | GTO   | $1\sigma_\alpha (1\sigma 2\sigma 3\sigma)_\beta$   | $0 \leq B < 0.2$         |
|            |       | $1\sigma_\alpha (1\sigma 2\sigma 1\pi)_\beta$      | $0.2 \leq B < 2.1$       |
|            |       | $1\sigma_\alpha (1\sigma 1\pi 2\sigma)_\beta$      | $2.1 \leq B \leq 10$     |
|            |       |                                                    |                          |
| quintet    | FEM   | $(1\sigma 2\sigma 3\sigma 1\pi)_\beta$             | $0 \leq B \leq 0.1$      |
|            |       | $(1\sigma 2\sigma 1\pi 3\sigma)_\beta$             | $0.1 < B < 1.3$          |
|            |       | $(1\sigma 1\pi 2\sigma 3\sigma)_\beta$             | $1.3 \leq B < 1.5$       |
|            |       | $(1\sigma 1\pi 2\sigma 1\delta)_\beta$             | $1.5 \leq B < 5.8$       |
|            |       | $(1\sigma 1\pi 1\delta 2\sigma)_\beta$             | $5.8 \leq B \leq 10$     |
|            | GTO   | $(1\sigma 2\sigma 3\sigma 1\pi)_\beta$             | $0 \leq B < 0.2$         |
|            |       | $(1\sigma 2\sigma 1\pi 3\sigma)_\beta$             | $0.2 \leq B < 1.3$       |
|            |       | $(1\sigma 1\pi 2\sigma 3\sigma)_\beta$             | $1.3 \leq B \leq 10$     |
|            |       |                                                    |                          |



Table 3.: Ground-state configurations for BH as a function of the magnetic field strength calculated at the Hartree–Fock level using gauge-including Gaussian-type orbitals (GTO) and finite element (FEM) basis sets.  $\pi_+$  orbitals have a higher energy in the presence of the magnetic field than at zero field.

| Spin state | basis | configuration                                                      | field strength ( $B_0$ ) |
|------------|-------|--------------------------------------------------------------------|--------------------------|
| singlet    | FEM   | $(1\sigma 2\sigma 3\sigma)_\alpha (1\sigma 2\sigma 3\sigma)_\beta$ | $0 \leq B < 0.3$         |
|            |       | $(1\sigma 2\sigma 1\pi)_\alpha (1\sigma 2\sigma 1\pi)_\beta$       | $0.3 \leq B < 0.9$       |
|            |       | $(1\sigma 1\pi 2\sigma)_\alpha (1\sigma 1\pi 2\sigma)_\beta$       | $0.9 \leq B \leq 10$     |
|            | GTO   | $(1\sigma 2\sigma 3\sigma)_\alpha (1\sigma 2\sigma 3\sigma)_\beta$ | $0 \leq B < 0.3$         |
|            |       | $(1\sigma 2\sigma 1\pi)_\alpha (1\sigma 2\sigma 1\pi)_\beta$       | $0.3 \leq B < 0.7$       |
|            |       | $(1\sigma 1\pi 2\sigma)_\alpha (1\sigma 1\pi 2\sigma)_\beta$       | $0.7 \leq B \leq 10$     |
| triplet    | FEM   | $(1\sigma 2\sigma)_\alpha (1\sigma 2\sigma 3\sigma 1\pi)_\beta$    | $0 \leq B < 0.3$         |
|            |       | $(1\sigma 2\sigma)_\alpha (1\sigma 2\sigma 1\pi 3\sigma)_\beta$    | $0.3 \leq B < 0.9$       |
|            |       | $(1\sigma 2\sigma)_\alpha (1\sigma 1\pi 2\sigma 3\sigma)_\beta$    | $0.9 \leq B < 1.2$       |
|            |       | $(1\sigma 1\pi)_\alpha (1\sigma 2\sigma 1\pi 3\sigma)_\beta$       | $1.2 \leq B < 2.7$       |
|            |       | $(1\sigma 1\pi)_\alpha (1\sigma 1\pi 2\sigma 3\sigma)_\beta$       | $2.7 \leq B < 3.6$       |
|            |       | $(1\sigma 1\pi)_\alpha (1\sigma 1\pi 2\sigma 2\pi)_\beta$          | $3.6 \leq B \leq 10$     |
|            | GTO   | $(1\sigma 2\sigma)_\alpha (1\sigma 2\sigma 3\sigma 1\pi)_\beta$    | $0 \leq B < 0.3$         |
|            |       | $(1\sigma 2\sigma)_\alpha (1\sigma 2\sigma 1\pi 3\sigma)_\beta$    | $0.3 \leq B < 0.9$       |
|            |       | $(1\sigma 2\sigma)_\alpha (1\sigma 1\pi 2\sigma 3\sigma)_\beta$    | $0.9 \leq B < 1.5$       |
|            |       | $(1\sigma 1\pi)_\alpha (1\sigma 2\sigma 1\pi 3\sigma)_\beta$       | $1.5 \leq B < 3.3$       |
|            |       | $(1\sigma 1\pi)_\alpha (1\sigma 1\pi 2\sigma 3\sigma)_\beta$       | $3.3 \leq B \leq 10$     |
|            |       |                                                                    |                          |
| quintet    | FEM   | $1\sigma_\alpha (1\sigma 2\sigma 3\sigma 1\pi 1\pi_+)_\beta$       | $0 \leq B < 0.3$         |
|            |       | $1\sigma_\alpha (1\sigma 2\sigma 1\pi 3\sigma 1\pi_+)_\beta$       | $B = 0.3$                |
|            |       | $1\sigma_\alpha (1\sigma 2\sigma 1\pi 3\sigma 1\delta)_\beta$      | $0.4 \leq B < 1.5$       |
|            |       | $1\sigma_\alpha (1\sigma 1\pi 2\sigma 3\sigma 1\delta)_\beta$      | $1.5 \leq B < 1.8$       |
|            |       | $1\sigma_\alpha (1\sigma 1\pi 2\sigma 1\delta 3\sigma)_\beta$      | $1.8 \leq B \leq 10$     |
|            |       |                                                                    |                          |
|            | GTO   | $1\sigma_\alpha (1\sigma 2\sigma 3\sigma 1\pi 1\pi_+)_\beta$       | $0 \leq B < 0.4$         |
|            |       | $1\sigma_\alpha (1\sigma 2\sigma 3\sigma 4\sigma 1\pi)_\beta$      | $0.4 \leq B < 0.7$       |
|            |       | $1\sigma_\alpha (1\sigma 2\sigma 3\sigma 1\pi 2\pi)_\beta$         | $0.7 \leq B < 1.5$       |
|            |       | $1\sigma_\alpha (1\sigma 1\pi 2\sigma 3\sigma 1\delta)_\beta$      | $1.5 \leq B < 2.0$       |
|            |       | $1\sigma_\alpha (1\sigma 1\pi 2\sigma 1\delta 3\sigma)_\beta$      | $2.0 \leq B < 3.3$       |
|            |       | $1\sigma_\alpha (1\sigma 1\pi 2\sigma 3\sigma 1\delta)_\beta$      | $3.3 \leq B < 4.0$       |
|            |       | $1\sigma_\alpha (1\sigma 2\sigma 3\sigma 4\sigma 1\pi)_\beta$      | $4.0 \leq B \leq 10$     |

Table 4.: Ground-state configurations for  $\text{CH}^+$  as a function of the magnetic field strength calculated at the Hartree–Fock level using gauge-including Gaussian-type orbitals (GTO) and finite element (FEM) basis sets.  $\pi_+$  orbitals have a higher energy in the presence of the magnetic field than at zero field.

| Spin state | basis | configuration                                                      | field strength ( $B_0$ ) |
|------------|-------|--------------------------------------------------------------------|--------------------------|
| singlet    | FEM   | $(1\sigma 2\sigma 3\sigma)_\alpha (1\sigma 2\sigma 3\sigma)_\beta$ | $0 \leq B < 0.3$         |
|            |       | $(1\sigma 2\sigma 1\pi)_\alpha (1\sigma 2\sigma 1\pi)_\beta$       | $0.3 \leq B < 1.0$       |
|            |       | $(1\sigma 1\pi 2\sigma)_\alpha (1\sigma 1\pi 2\sigma)_\beta$       | $1.0 \leq B \leq 10$     |
|            | GTO   | $(1\sigma 2\sigma 3\sigma)_\alpha (1\sigma 2\sigma 3\sigma)_\beta$ | $0 \leq B < 0.3$         |
|            |       | $(1\sigma 2\sigma 1\pi)_\alpha (1\sigma 2\sigma 1\pi)_\beta$       | $0.3 \leq B < 1.0$       |
|            |       | $(1\sigma 1\pi 2\sigma)_\alpha (1\sigma 1\pi 2\sigma)_\beta$       | $1.0 \leq B \leq 10$     |
| triplet    | FEM   | $(1\sigma 2\sigma)_\alpha (1\sigma 2\sigma 3\sigma 1\pi)_\beta$    | $0 \leq B < 0.3$         |
|            |       | $(1\sigma 2\sigma)_\alpha (1\sigma 2\sigma 1\pi 3\sigma)_\beta$    | $0.3 \leq B < 1.0$       |
|            |       | $(1\sigma 2\sigma)_\alpha (1\sigma 1\pi 2\sigma 3\sigma)_\beta$    | $B = 1.0$                |
|            |       | $(1\sigma 1\pi)_\alpha (1\sigma 2\sigma 1\pi 3\sigma)_\beta$       | $1.1 \leq B < 1.5$       |
|            |       | $(1\sigma 1\pi)_\alpha (1\sigma 1\pi 2\sigma 3\sigma)_\beta$       | $1.5 \leq B \leq 10$     |
|            |       | $(1\sigma 1\pi)_\alpha (1\sigma 1\pi 2\sigma 3\sigma)_\beta$       | $1.5 \leq B \leq 10$     |
|            | GTO   | $(1\sigma 2\sigma)_\alpha (1\sigma 2\sigma 3\sigma 1\pi)_\beta$    | $0 \leq B < 0.3$         |
|            |       | $(1\sigma 2\sigma)_\alpha (1\sigma 2\sigma 1\pi 3\sigma)_\beta$    | $0.3 \leq B < 1.0$       |
|            |       | $(1\sigma 2\sigma)_\alpha (1\sigma 1\pi 2\sigma 3\sigma)_\beta$    | $1.0 \leq B < 1.3$       |
|            |       | $(1\sigma 1\pi)_\alpha (1\sigma 2\sigma 1\pi 3\sigma)_\beta$       | $1.3 \leq B < 1.5$       |
|            |       | $(1\sigma 1\pi)_\alpha (1\sigma 1\pi 2\sigma 3\sigma)_\beta$       | $1.5 \leq B \leq 10$     |
|            |       | $(1\sigma 1\pi)_\alpha (1\sigma 1\pi 2\sigma 3\sigma)_\beta$       | $1.5 \leq B \leq 10$     |
| quintet    | FEM   | $1\sigma_\alpha (1\sigma 2\sigma 3\sigma 1\pi 1\pi_+)_\beta$       | $0 \leq B < 0.3$         |
|            |       | $1\sigma_\alpha (1\sigma 2\sigma 1\pi 3\sigma 1\pi_+)_\beta$       | $0.3 \leq B < 0.7$       |
|            |       | $1\sigma_\alpha (1\sigma 2\sigma 1\pi 3\sigma 1\delta)_\beta$      | $0.7 \leq B < 1.2$       |
|            |       | $1\sigma_\alpha (1\sigma 1\pi 2\sigma 3\sigma 1\delta)_\beta$      | $1.2 \leq B < 3.0$       |
|            |       | $1\sigma_\alpha (1\sigma 1\pi 2\sigma 1\delta 3\sigma)_\beta$      | $3.0 \leq B < 6.6$       |
|            |       | $1\sigma_\alpha (1\sigma 1\pi 1\delta 2\sigma 3\sigma)_\beta$      | $6.6 \leq B \leq 10$     |
|            | GTO   | $1\sigma_\alpha (1\sigma 2\sigma 3\sigma 1\pi 1\pi_+)_\beta$       | $0 \leq B < 0.3$         |
|            |       | $1\sigma_\alpha (1\sigma 2\sigma 1\pi 3\sigma 1\pi_+)_\beta$       | $0.3 \leq B < 0.7$       |
|            |       | $1\sigma_\alpha (1\sigma 2\sigma 1\pi 3\sigma 1\delta)_\beta$      | $0.7 \leq B < 1.2$       |
|            |       | $1\sigma_\alpha (1\sigma 1\pi 2\sigma 3\sigma 1\delta)_\beta$      | $1.2 \leq B < 3.4$       |
|            |       | $1\sigma_\alpha (1\sigma 1\pi 2\sigma 1\delta 3\sigma)_\beta$      | $3.4 \leq B < 6.5$       |
|            |       | $1\sigma_\alpha (1\sigma 2\sigma 3\sigma 4\sigma 1\pi)_\beta$      | $6.5 \leq B \leq 10$     |
